# Supplementary material for: Linear Scaling Calculations of Excitation Energies with Active-Space Particle-Particle Random Phase Approximation
Source: arXiv:2305.00369 ancillary file (2023-04-30)
Supplement: Supplementary file 1 [file supporting_information.pdf]

# Supporting Information: Linear Scaling Calculations of Excitation Energies with Active-Space Particle-Particle Random Phase Approximation

Jiachen Li, Jincheng Yu, Zehua Chen, and Weitao Yang*

*Department of Chemistry, Duke University, Durham, NC 27708, USA*

E-mail: weitao.yang@duke.edu

## 1 Convergence behavior of the active-space T-matrix approach

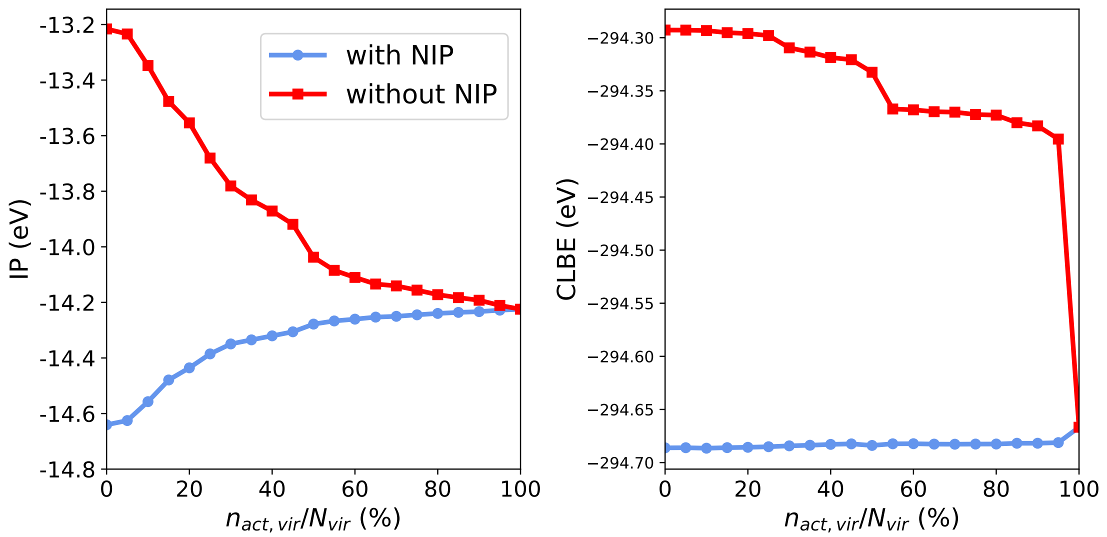


Figure S1: Comparisons of ionization potential (left) and core-level bind energy (right) of $CH_4$ obtained from the active-space $G_0T_0$@HF approach with different sizes of the active space. The active spaces include all occupied orbitals and different numbers of virtual orbitals. The def2-TZVPP basis set was used.

## 2 Core-level binding energies obtained from $G_0T_0$ and $G_{\mathrm{RS}}T_{\mathrm{RS}}$

Table S1: Core-level binding energies of a subset of the CORE65[S1] set obtained from $G_0T_0$ and $G_{\mathrm{RS}}T_{\mathrm{RS}}$ based on HF, PBE and B3LYP. The def2-TZVP basis set was used. All values in eV.

| | | | $G_0T_0$ | | | $G_{\mathrm{RS}}T_{\mathrm{RS}}$ | | |
|---|---|---|---|---|---|---|---|---|
| molecule | core level | ref | HF | PBE | B3LYP | HF | PBE | B3LYP |
| $CH_4$ | C1s | 290.844 | 294.78 | 280.13 | 284.50 | 294.78 | 292.27 | 292.31 |
| $C_2H_6$ | C1s | 290.714 | 294.56 | 279.43 | 283.97 | 294.56 | 292.42 | 292.54 |
| $C_2H_4$ | C1s | 290.823 | 295.00 | 278.85 | 283.77 | 295.00 | 292.72 | 292.85 |
| $C_2H_2$ | C1s | 291.249 | 295.18 | 279.01 | 283.95 | 295.18 | 293.03 | 293.17 |

Table S1: Continued

| molecule | core level | ref | $G_0T_0$ | | | $G_{RS}T_{RS}$ | | |
|---|---|---|---|---|---|---|---|---|
| | | | HF | PBE | B3LYP | HF | PBE | B3LYP |
| CO | O1s | 542.1 | 545.11 | | | 545.11 | 543.66 | 543.50 |
| CO | C1s | 296.229 | 300.59 | | | 300.59 | 298.17 | 298.50 |
| $CO_2$ | O1s | 541.32 | 544.50 | 522.04 | | 544.50 | 542.36 | 542.41 |
| $CO_2$ | C1s | 297.699 | 302.72 | 286.19 | | 302.72 | 298.76 | 299.57 |
| $CF_4$ | F1s | 695.2 | 698.43 | 675.77 | 682.88 | 698.43 | 696.82 | 696.57 |
| $CF_4$ | C1s | 301.898 | 306.36 | 289.83 | 295.05 | 306.36 | 302.65 | 303.42 |
| $CFH_3$ | F1s | 692.4 | 695.38 | 673.41 | 680.12 | 695.38 | 694.28 | 694.03 |
| $CFH_3$ | C1s | 293.557 | 297.69 | 282.68 | 287.29 | 297.69 | 295.46 | 295.69 |
| $CF_3H$ | F1s | 694.1 | 697.48 | 674.87 | 682.11 | 697.48 | 696.08 | 695.94 |
| $CF_3H$ | C1s | 299.159 | 303.61 | 287.64 | 292.67 | 303.61 | 300.39 | 300.99 |
| $CH_3OH$ | O1s | 538.88 | 542.06 | 521.87 | 527.93 | 542.06 | 540.45 | 540.29 |
| $CH_3OH$ | C1s | 292.3 | 296.44 | 281.36 | 285.95 | 296.44 | 294.28 | 294.47 |
| $CH_2O$ | O1s | 539.33 | 542.40 | | 527.47 | 542.40 | 540.88 | 540.71 |
| $CH_2O$ | C1s | 294.38 | 298.88 | | 288.25 | 298.88 | 296.42 | 296.73 |
| $CH_3{-}O{-}CH_3$ | O1s | 538.36 | 541.57 | 520.75 | 526.55 | 541.57 | 540.04 | 539.83 |
| $CH_3{-}O{-}CH_3$ | C1s | 292.17 | 296.28 | 280.83 | 285.58 | 296.28 | 294.05 | 294.25 |
| HCOOH | O1s OH | 540.69 | 543.94 | 522.47 | 528.52 | 543.94 | 542.08 | 542.00 |
| HCOOH | O1s C=O | 539.02 | 542.08 | 520.13 | 526.86 | 542.08 | 540.30 | 540.23 |
| HCOOH | C1s | 295.75 | 300.23 | 284.17 | 289.23 | 300.23 | 297.21 | 297.73 |
| $CH_3CO_2H$ | O1s OCH3 | 539.64 | 543.06 | | 527.53 | 543.06 | 541.24 | 541.10 |
| $CH_3CO_2H$ | O1s C=O | 538.24 | 541.76 | | 526.42 | 541.76 | 539.94 | 539.87 |
| $CH_3COOH$ | O1s OH | 540.10 | 543.49 | 521.99 | 528.24 | 543.49 | 541.55 | 541.48 |
| $CH_3COOH$ | O1s C=O | 538.31 | 541.51 | 519.51 | 526.23 | 541.51 | 539.68 | 539.62 |
| $CH_3COOH$ | C1s COOH | 295.35 | 299.74 | 283.10 | 288.25 | 299.74 | 296.62 | 297.11 |
| $CH_3COOH$ | C1s CH3 | 291.55 | 295.47 | 280.06 | 284.89 | 295.47 | 293.44 | 293.59 |
| $H_2O$ | O1s | 539.7 | 542.90 | | 529.16 | 542.90 | 541.45 | 541.31 |
| $O_3$ | O1s middle | 546.44 | 551.09 | | 534.25 | 551.09 | | 548.07 |
| $O_3$ | O1s terminal | 541.75 | 545.43 | | 527.67 | 545.43 | | 542.81 |
| $N_2$ | N1s | 409.93 | 413.52 | 394.80 | | 413.52 | 411.22 | 411.38 |
| $NH_3$ | N1s | 405.52 | 409.18 | 391.85 | 396.85 | 409.18 | 407.32 | 407.26 |
| HCN | N1s | 406.8 | 410.45 | 390.81 | | 410.45 | 408.32 | 408.37 |

Table S1: Continued

| | | | $G_0T_0$ | | | $G_{\mathrm{RS}}T_{\mathrm{RS}}$ | | |
|---|---|---|---|---|---|---|---|---|
| molecule | core level | ref | HF | PBE | B3LYP | HF | PBE | B3LYP |
| HCN | C1s | 293.5 | 297.24 | 281.89 | | 297.24 | 295.07 | 295.28 |
| $CH_3CN$ | N1s | 405.58 | 409.46 | 389.31 | 395.17 | 409.46 | 407.30 | 407.44 |
| $CH_3CN$ | C1s CH3 | 292.88 | 296.70 | 280.63 | 285.77 | 296.70 | 294.40 | 294.57 |
| $CH_3CN$ | C1s CN | 292.60 | 296.44 | 280.70 | 285.57 | 296.44 | 294.19 | 294.44 |
| $CO(NH_2)_2$ | O1s | 537.19 | 540.46 | 518.40 | 525.12 | 540.46 | 538.60 | 538.52 |
| $CO(NH_2)_2$ | N1s | 406.09 | 409.89 | 391.14 | 396.80 | 409.89 | 407.80 | 407.80 |
| $CO(NH_2)_2$ | C1s | 294.84 | 299.31 | 282.63 | 287.72 | 299.31 | 296.04 | 296.57 |
| $CH_3NH_2$ | N1s | 405.17 | 408.73 | 390.76 | 395.99 | 408.73 | 406.87 | 406.79 |
| $O_2$ | O1s up | 544.2 | 547.59 | | 531.90 | 547.59 | | 545.44 |
| $O_2$ | O1s down | 543.1 | 547.50 | | 531.87 | 547.50 | | 545.39 |
| $(CH_3)_2CO$ | O1s | 537.73 | 541.25 | 519.13 | 525.88 | 541.25 | 539.50 | 539.40 |
| $(CH_3)_2CO$ | C1s C=O | 293.88 | 297.82 | 281.36 | 286.48 | 297.82 | 295.22 | 295.52 |
| $(CH_3)_2CO$ | C1s CH3 | 291.23 | 295.15 | 279.41 | 284.32 | 295.15 | 292.88 | 293.16 |
| $C_2H_5NO_2$ | O1s OH | 540.2 | 543.62 | 521.87 | 528.35 | 543.62 | 541.64 | 541.55 |
| $C_2H_5NO_2$ | O1s C=O | 538.4 | 541.67 | 519.55 | 526.32 | 541.67 | 539.83 | 539.77 |
| $C_2H_5NO_2$ | N1s | 405.4 | 409.17 | 390.81 | 396.31 | 409.17 | 407.25 | 407.20 |
| $C_2H_5NO_2$ | C1s COOH | 295.2 | 299.59 | 282.67 | 287.93 | 299.59 | 296.40 | 296.97 |
| $C_2H_5NO_2$ | C1s CH2 | 292.3 | 296.16 | 280.23 | 285.18 | 296.16 | 293.89 | 294.08 |
| $C_5H_5N$ | N1s | 404.82 | 408.72 | 388.21 | 394.09 | 408.72 | 406.22 | 406.29 |
| $C_4H_4NH$ | N1s | 406.18 | 409.66 | | 396.19 | 409.66 | 407.65 | 407.59 |
| $C_6H_5NH_2$ | N1s | 405.31 | 409.10 | 388.52 | 395.56 | 409.10 | 407.15 | 407.08 |
| $C_6H_5NO_2$ | O1s | 538.63 | 542.54 | | 525.68 | 542.54 | 540.23 | 540.29 |
| $C_6H_5NO_2$ | N1s | 411.6 | 416.58 | | 401.06 | 416.58 | 412.81 | 413.16 |
| $C_6H_5NO_2$ | C1s C1 | 292.08 | 296.04 | | 283.60 | 296.04 | 293.57 | 293.76 |
| $C_6H_5NO_2$ | C1s C234 | 291.13 | 295.36 | | 283.09 | 295.36 | 292.92 | 293.11 |
| $C_6H_6$ | C1s | 290.377 | 294.31 | 276.99 | 282.39 | 294.31 | 292.08 | 292.23 |
| $C_8H_6$ | C1s C3 | 290.88 | 294.72 | 276.97 | 282.44 | 294.72 | 292.51 | 292.65 |
| $C_8H_6$ | C1s C2 | 290.55 | 294.47 | 276.73 | 282.44 | 294.47 | 292.26 | 292.40 |
| $C_8H_6$ | C1s C456 | 290.16 | 294.45 | 276.52 | 282.14 | 294.45 | 292.11 | 292.34 |
| $C_8H_6$ | C1s C1 | 289.75 | 294.49 | 281.02 | 282.29 | 294.49 | 292.16 | 292.34 |

# References

(S1) Golze, D.; Keller, L.; Rinke, P. Accurate Absolute and Relative Core-Level Binding Energies from GW. *J. Phys. Chem. Lett.* **2020**, *11*, 1840–1847.
